# Supplementary material for: ReStyle3D: Scene-Level Appearance Transfer with Semantic Correspondences
Source: arXiv:2502.10377 source file (2025-04-25)
Supplement: Supplementary file 1 [file 7_appendix.tex]

\clearpage
\appendix
In this supplementary material we provide:
\begin{itemize}
\item A video (\texttt{supplementary.mp4}) explaining our main paper with additional qualitative \textit{video} results
\item The template of our user study (\texttt{user\_study.pdf})
\item A qualitative ablation study (Sec.~\ref{sec:qual_ablation}),
\item Additional qualitative results (Sec.~\ref{sec:more_quals})
\item Details on the data curation (Sec.~\ref{sec:train_data})
\item Samples of the collected style images along with semantic segmentation results (Sec.~\ref{sec:design_style})
\item Limitations and future work (Sec.~\ref{sec:limitation})
\end{itemize}

\section{Qualitative Ablation Study}
\label{sec:qual_ablation}
\begin{figure*}[t]
\begin{center}
\centering
\includegraphics[width=0.85\linewidth]{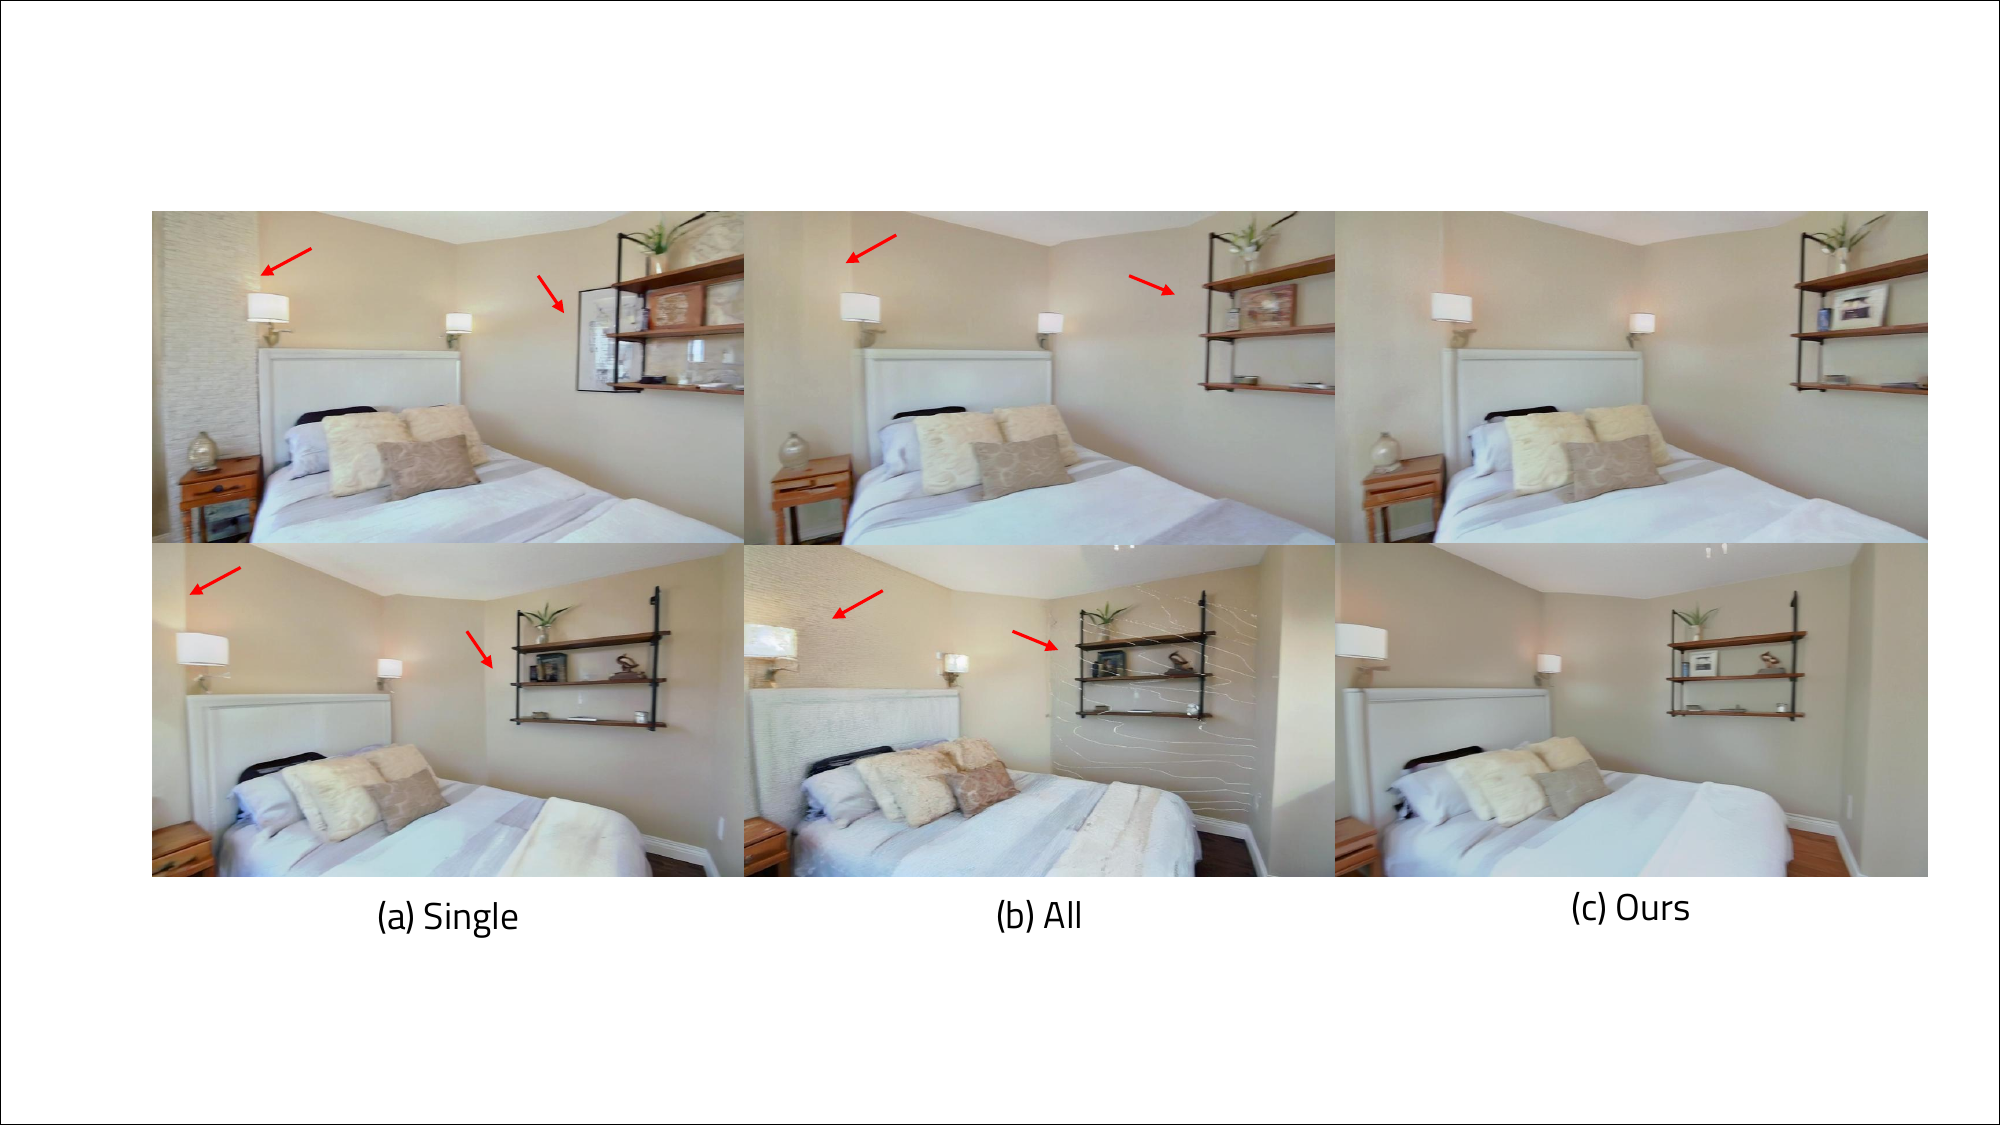}
\end{center}
% \vspace{-15pt}
\caption{
\textbf{Comparison between different auto-regression strategies.} The rows represent two non-sequential views used in multi-view appearance transfer, while the columns represent different frame selection strategies. (a) \textit{Single} warps only the previous view, failing to preserve details like the painting on the wall present in the top image, as pixel information is lost. (b) \textit{All} warps all past frames to the current frame, improving consistency but introducing smearing effects, demonstrated by the red arrows (highlighted by red arrows) due to overlapping pixel projections with large color value differences originating from lighting changes. (c) \textit{Ours}, the proposed strategy in \ours, achieves the most consistent and clean multi-view stylization.
}
% \vspace{-15pt}
\label{fig:ar_ablation}
\end{figure*}

\vspace{15pt}

\begin{figure*}[t]
\begin{center}
\centering
\includegraphics[width=0.99\linewidth]{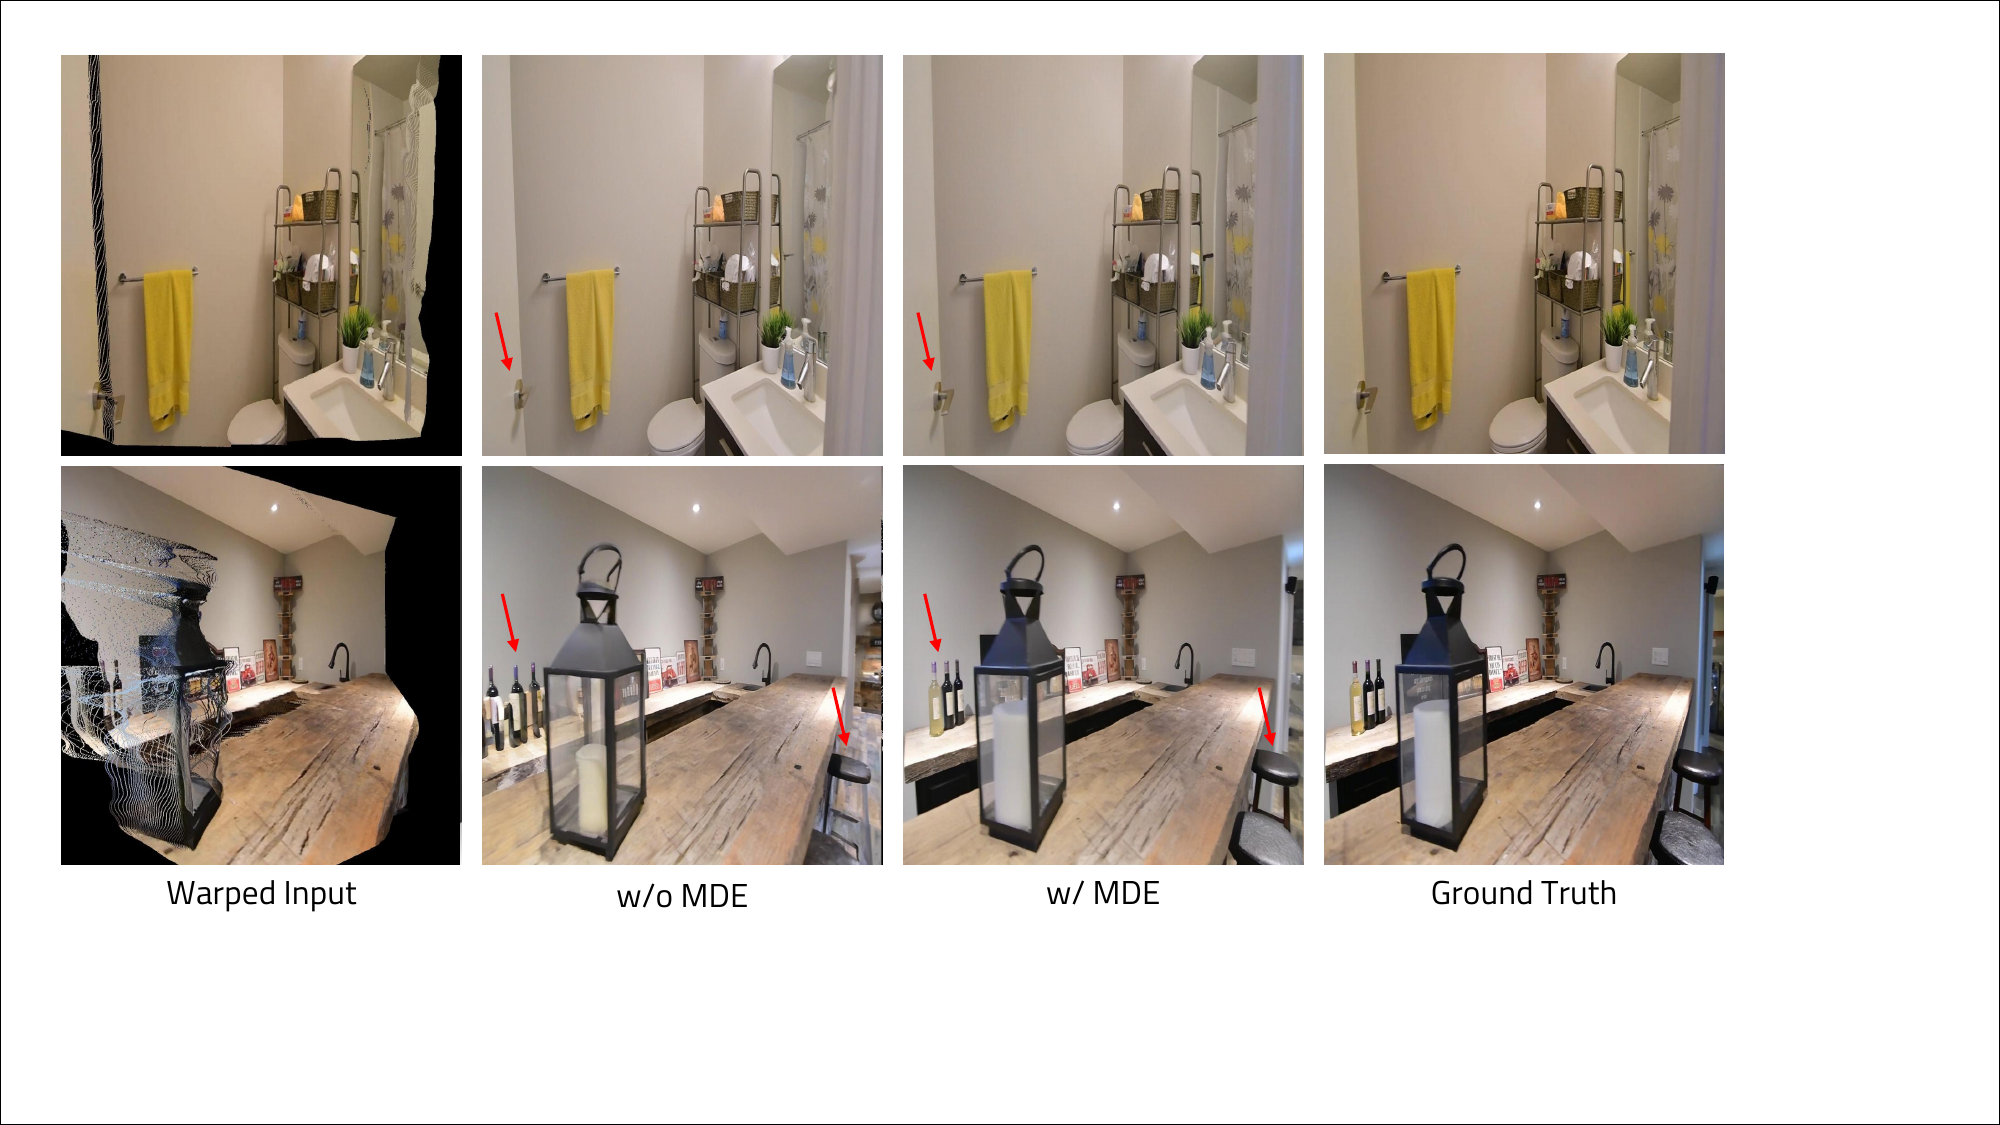}
\end{center}
% \vspace{-15pt}
\caption{
\textbf{Qualitative comparison between two different conditional models.}  We train a warp-and-refine model without the monocular depth~(MDE) condition. Without MDE supervision, the model struggles to correct local alignment issues~(\eg, the door handle, wine bottles, and chairs), resulting in noticeable geometric distortions and texture artifacts. In contrast, incorporating MDE enables the model to leverage pixel-aligned depth cues and more faithfully reconstruct fine details, yielding sharper and more consistent multi-view results.
}
% \vspace{-15pt}
\label{fig:qualitative_ablation}
\end{figure*}
% Fig.~\ref{fig:qualitative_ablation} demonstrates the qualitative ablations of our method. Results show that ...
We further validate our design choices with additional qualitative results in Fig.~\ref{fig:ar_ablation}, comparing frame selection strategies for our warp-and-refine model.
Warping only the last frame can cause inconsistencies, \eg, the painting on the wall appears and disappears due to occlusion and incorrect correspondence estimates (Fig.~\ref{fig:ar_ablation} (a)).
Warping all past frames improves consistency but introduces conflicts, as overlapping pixel projections in the same location can result in smeared pixels and confuse the model about whether to refine or preserve them (Fig.~\ref{fig:ar_ablation} (b)).
Our strategy can mitigate the disadvantages of both approaches, yielding more coherent multi-view stylization (Fig.~\ref{fig:ar_ablation} (c)). 

We also validate the need for monocular depth condition to fully leverage two-view geometry in multi-view appearance transfer. As the stereo estimate from DUSt3R~\cite{wang2024dust3r} implicitly contains geometry information, the additional monocular depth condition could be deemed unnecessary. To this end, we train a model without monocular depth estimation (MDE) that is solely conditioned on warped images, to ablate its effect.
Fig.~\ref{fig:qualitative_ablation} shows that without MDE, the model still effectively learns the task, but loses fidelity in local details.
With pixel-aligned MDE control, the model corrects wrong projections from two-view geometry based on the high-resolution depth map improving accuracy in areas like the door handle, chairs, and wine bottles.

\section{Qualitative Video Results}
\label{sec:more_quals}
We present additional results that demonstrate our method's versatility in handling diverse styles and scene contents. Our supplemental video best illustrates this versatility, showing how a single style image can transform multiple indoor scenes into a cohesive appearance, as well as how one scene can be re-imagined across various styles. The video format particularly highlights our method's ability to maintain visual consistency across multiple viewpoints, a key advantage that is difficult to convey through static images.

\section{Data Curation}
\label{sec:train_data}
We curated the training data for our warp-and-refine model using 57 hourly-long 2K house tour videos \cite{housetour}. We first extract keyframes from all the videos at every 10$^{th}$ frame to get 57K sparse multi-view images. Then we divide the keyframes into 10-image chunks to emulate different overlap ratios in real-world scenarios. In each window, we use DUSt3R~\cite{wang2024dust3r} to compute the dense stereo between the first frame in the window and the rest of the frames, resulting to 9 warped images and their warping masks in each window. We also use Depth Anything V2~\cite{yang2024depth} to extract the monocular depth for the 9$^{th}$ image in the window. Then each training sample is generated as (warped image, monocular depth, mask, and clean target image) and used for training. 

We would like to note that both the warp-and-refine training data and the \dataset benchmark data are derived from the same collection of house tour videos \cite{housetour}. The selection of this dataset was intentional. Unlike existing indoor scene datasets~\cite{dai2017scannet,yeshwanth2023scannet++}, which are typically designed for 3D reconstruction and feature imagery that remains close to surfaces and lacks spatial context, our house tour videos were collected for real-estate purposes. They offer stable, smooth trajectories with views that are further from surfaces, making them more suitable for stylization tasks.

The style images in the \dataset benchmark were manually collected from \href{https://www.pexels.com/search/interior%20design/}{\textit{Pexels Interior Design Image Collection}}, which provides copyright-free interior images.

\section{Style Images and Segmentation}
\label{sec:design_style}
\begin{figure*}[t]
\begin{center}
\centering
\includegraphics[width=0.99\linewidth]{figures/images/style_examples.pdf}
\end{center}
% \vspace{-15pt}
\caption{
\textbf{Style Image Samples. }We showcase exemplar images of various designs across various styles and types of rooms from our \dataset benchmark style image collection~(top rows), paired with their open-vocabulary semantic segmentation masks~(bottom rows). These images span a variety of interior spaces--including kitchens, living rooms, and bedrooms--and illustrate the core challenge of \ours: transferring the appearance of each semantically matched region~(e.g., cabinets, couches, and beds) from a style image to real-world 3D scenes. Our method leverages these semantic masks to ensure each object is stylized with the correct instance-level textures while maintaining photo-realism and multi-view consistency.
}
% \vspace{-15pt}
\label{fig:style_examples}
\end{figure*}
Fig~\ref{fig:style_examples} displays several style images from our \dataset benchmark alongside their open-vocabulary segmentation overlays.
Each row pairs a real indoor photograph~(kitchen, living room, or bedroom) with its corresponding color-coded semantic masks, as predicted by ODISE~\cite{xu2023open}.
The segmentation assigns each pixel to a semantic category~(e.g., ``wall'', ``sofa'', ``cabinet'', ``table'')\footnote{The open vocabulary method was queried with a list of common semantic labels. In our experiments we used the semantic list of the ODISE model.}, enabling instance-level alignment between the target scene and the reference style images.
In the \ours pipeline, these masks form the basis  for establishing precise semantic correspondences.
By ensuring that each object region in the target image only “borrows” style cues from its from its corresponding instance in the reference image, our framework preserves the scene layout while selectively transferring appearance.
This capability is particularly valuable in multi-object, complex scenes like the ones shown here, where various furniture and architectural elements must be stylized coherently while maintaining their original spatial relationships.
% In Fig.~\ref{fig:style_examples}, we showcase exemplar images and segmentation masks of various designs across various styles and types of rooms, paired with their open-vocabulary semantic segmentation masks~(bottom rows). These images span a variety of interior spaces—including kitchens, living rooms, and bedrooms—and illustrate the core challenge of ReStyle3D: transferring the appearance of each semantically matched region~(e.g., cabinets, sofas, beds) from a reference style image to real-world scenes. Our method leverages these semantic masks to ensure each object is stylized with the correct instance-level textures while maintaining photo-realism and multi-view consistency.

% \includepdf[pages=-]{figures/images/user_study}

\section{Limitations and Future Work}
\label{sec:limitation}
In this work we focused exclusively on indoor scenes for interior design applications, without exploring other types of scenes, such as outdoor or dynamic environments.
While our method effectively transfers appearance, it lacks strong disentanglement between color, texture, and material properties, and struggles with significant lighting changes.
Future work could address these limitations by improving the transfer of appearances for smaller objects in the scene---currently overlooked due to downsampling of semantic masks--- and developing finer control mechanism for appearance transfer, such as material or texture.
